# Supplementary material for: Enhancing Clinical Concept Extraction with Contextual Embeddings
Source: arXiv:1902.08691 source file (2019-08-14)
Supplement: Supplementary file 1 [file supplementary_material_ocz096.docx.pdf]

A. Supplemental Material

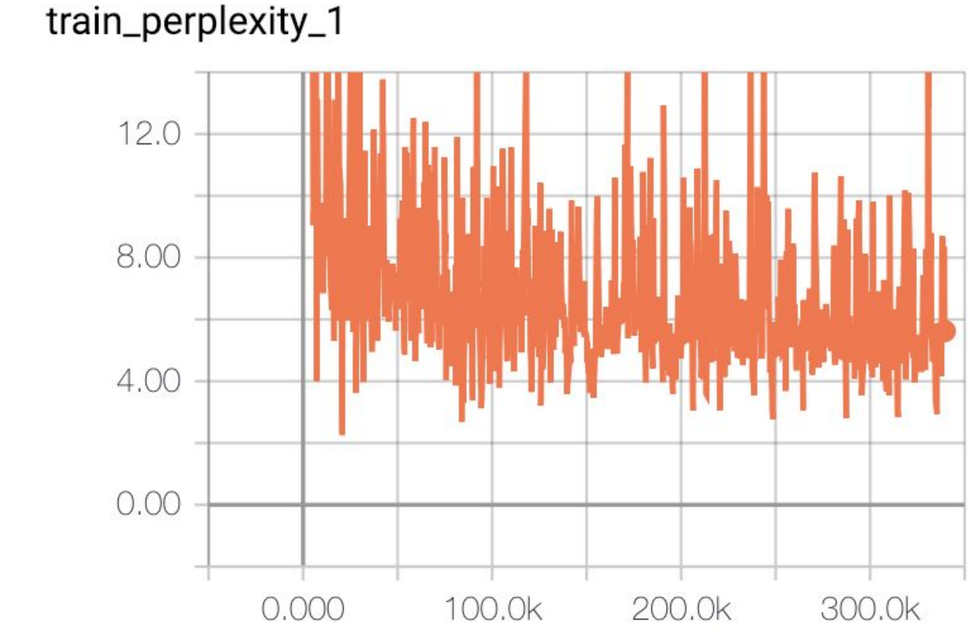


(a) ELMo (MIMIC)

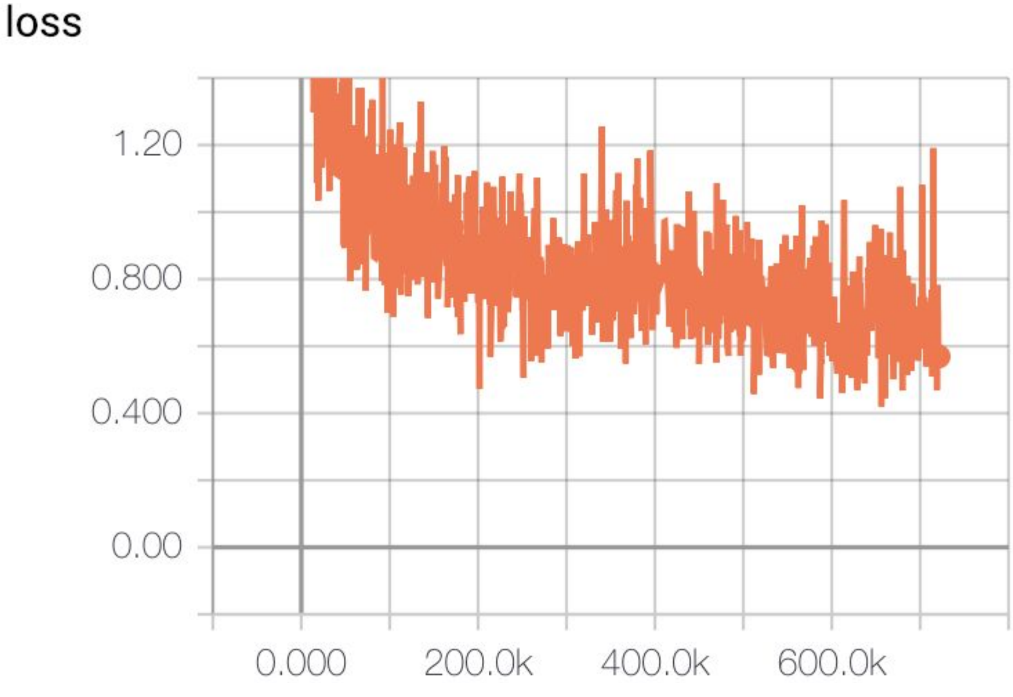


(b) $BERT_{BASE}$ (MIMIC)

Supplemental Figure 1: Training loss of language model over iteration steps.

# Supplemental Table 1: Sentences for PCA visualization

| | Web corpus | Clinical corpus |
|---|---|---|
| 1 | The woodman sang of the wild forest; the plowman sang of the fields; the shepherd sang of his sheep; and those who listened forgot about the storm and the cold weather. | Of note, her children, ages 2 and 5 months, have both had cold symptoms including fever, which started a few days before the patient ' s symptoms began. |
| 2 | He states he was in his usual state of health until 10: 30 last evening when he woke up feeling cold | he said he had cold symptoms. vomited several times. the throat may be affected |
| 3 | Cold is the presence of low temperature, | He does complain of cold symptoms times one week. |
| 4 | Its getting cold and colder because of the six horsemen of climate change | the patient stated that he had cold for 2 days prior to evaluation also nasal drainage, coughing. |
| 5 | What could be better on a cold winter's day than coming home to a fully cooked meal? | Guaifenesin 100mg/5ml Liquid Sig: 01-28 teaspoons P0 every six hours as needed for cold symptoms. |
| 6 | This time of year, when people are traveling and bouncing between hot and cold weather, | She reports that he stated that he was cold over the last few days with a mild cough. |
| 7 | I don't know how they get through these cold winters. | Did not try any cough / cold medications. |
| 8 | She always washes in cold water. | Cough that gets worse while other cold symptoms improve. |
| 9 | Slightly decreased sensation to temperature (cold) on dorsum of R foot between big toe and 2nd toe and decreased vibratory sense (3 seconds long) in toes bilaterally. | This patient ' s sudden onset sore throat, tender cervical lymphadenopathy, fever, and lack of cough or other symptoms of cold. |
| 10 | When your engine is cold, the gasoline is less likely to evaporate and create the correct ratio of air and vaporized fuel for combustion. | On admission, he noted several days of runny nose, sore throat, decreased PO intake, and feeling like he " had a cold." |
| 11 | This time of year, when people are traveling and bouncing between hot and cold weather, this is a favorite, and quite tasty, wintertime formula. | She had fullness in her ear and she also had a cold coinciding to the onset of her headache. |
| 12 | The water was too cold for swimming. | He states that around the same time, he developed a cold that involved sinus congestion and a cough. |
| 13 | Our hands may be cold, but at least our hearts are warm. | He gets cold easily but denies fevers. |
| 14 | The cold weather exhilarated the walkers. | Prior to onset of symptoms, she denied any recent local or foreign travel or cough / cold symptoms. |
| 15 | This month is the cold February in Los Angeles since 1962, with an average high temperature at 60.6 degrees as of Sunday, the National Weather Service said | Denies any urinary symptoms (no changes in color, consistency, dysuria, frequency, urgency) , abd pain , neck stiffness , cough or cold symptoms. |
| 16 | Temperature is degree of hotness or cold ness as measured on a scale. | 2 months ago, the patient first caught a cold with a sore throat, bad taste in back of throat, and DOE. |
| 17 | The nights were still cold into April, but the temperature climbed into the 60 during the day. | There were no preceding illnesses including cough, cold, vomiting, diarrhea or fever. |
| 18 | Who knows how long the cold weather will last? | The patient uses nsaids once in awhile when he has a cold. |
| 19 | In a very cold night, even houses want to have houses of their own to enter inside them and feel warm! | ROS: No fever, chills, cough, cold sx, CP, SOB, abdominal pain. |
| 20 | In cold weather it was no little amusement to bake several small loaves of this in succession, tending and turning them as carefully as an Egyptian his hatching eggs. | Dulcolax 10 mg Suppository Sig: One 1) supp Rectal once a day as needed for cold symptoms. |
| 21 | A severe cold of a few days duration in March may very much retard the opening of the former ponds, while the temperature of Walden increases almost uninterruptedly. | For the past several weeks, she has had cold - like symptoms and post - nasal drip, but has been eating and drinking normally with normal activity levels. |
| 22 | Three feet of ice does not result from one day of cold weather. | Denies, coug, cold symptoms, fever, chills, nausea, vomiting, change in diet or medication. |
| 23 | States he was walking 1 mi / day prior to weather getting cold. | Patient initially attributed her discomfort to a cold. |
| 24 | Try to choose plants that live best with cold weather, and planting areas that face west. | She denied any nausea, vomiting, chills, feeling cold, and lightheadedness. |
| 25 | In cold weather, many of these volunteer firefighters wore coats made of the skin of buffalo to keep them warm and dry. | She also noted that she felt cold with shaking chills at the onset of the headache. |
| 26 | The unusually long period of cold weather has shown how even warm climates can sometimes freeze over. | 44 y / o with h / o HTN, s / p right thyroid lobectomy for benign adenoma presents with 5 days of cold symptoms. |
| 27 | Sensation: Intact to light touch, pinprick, temperature (cold), vibration, and proprioception. | The patient does attend a community center with elderly individuals and some have had cold. |
| 28 | Hot soup is the best because the process of digesting food helps to warm you up in cold weather like tonight. | I felt like I had a cold. my son brought me in, you should talk to him |
| 29 | Sensation: Decreased to light touch, temperature (cold), vibration on arm > leg. | Her cold then seemed to settle into her chest, with a sore throat predominating. |
| 30 | In the cold dark days of the winter, dream about the flowers to get warmed up | Denies any specific symptoms of illness - no cough or cold symptoms, no abd pain, diarrhea, vomiting. |

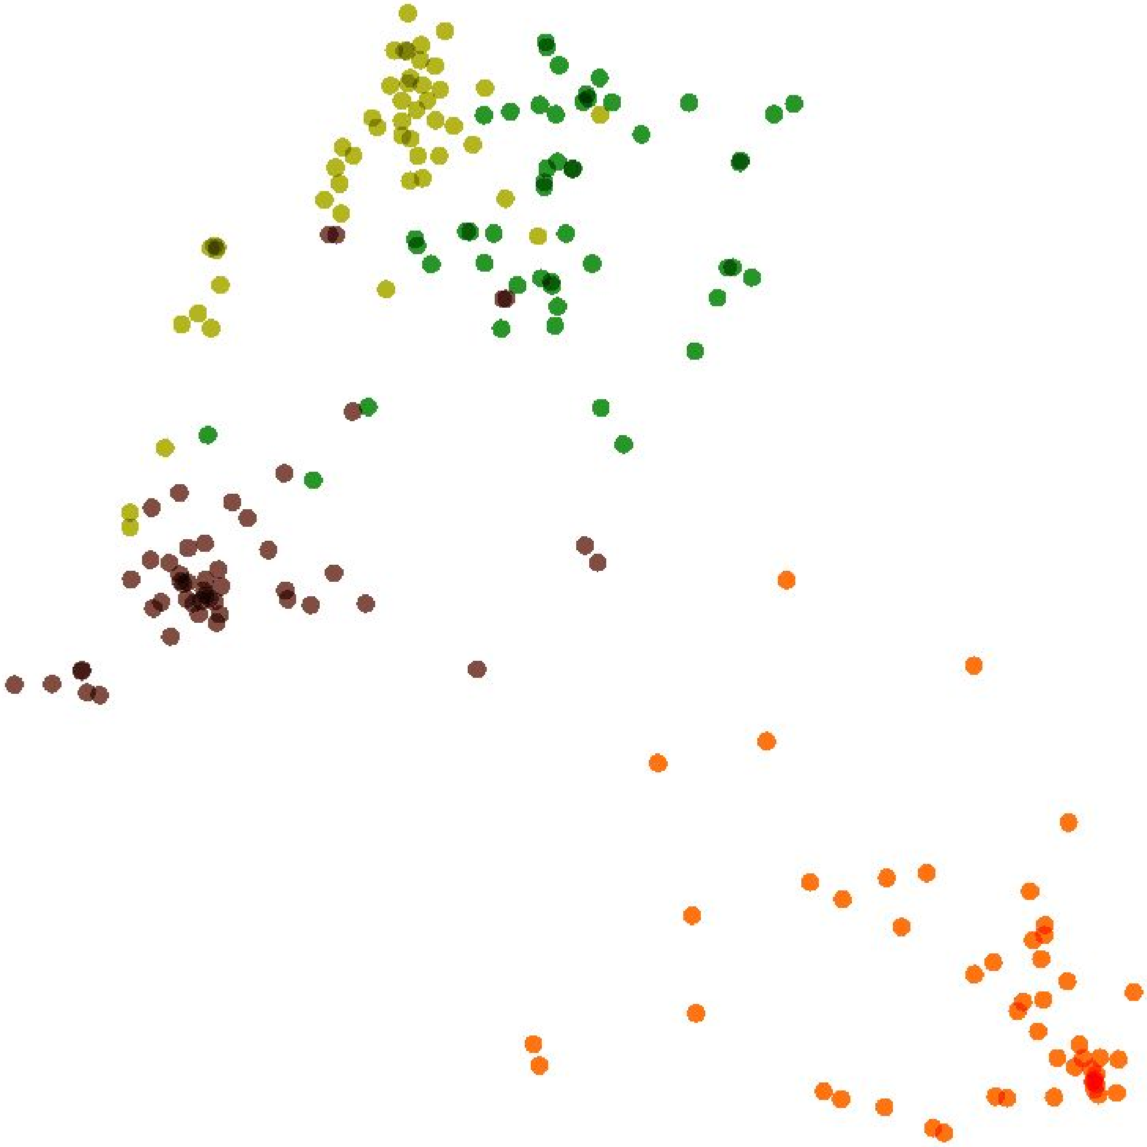

Supplemental Figure 2: PCA visualization for *tylenol* (olive), *motrin* (green), *pain* (brown), and *herpes* (orange).

Supplemental Table 2: Example word pieces for clinical terms.

| **Original Word** | **Word Piece Tokens** |
|---|---|
| acetylcysteine | ace, ##ty, ##l, ##cy, ##stein, ##e |
| acne | a, ##c, ##ne |
| activase | act, ##iva, ##se |
| actonel | act, ##one, ##l |
| adenitis | ad, ##eni, ##tis |
| adenosine | ad, ##eno, ##sin, ##e |
| agitation | agitation |
| agranulocytosis | a, ##gra, ##nu, ##loc, ##yt, ##osis |
| albumin | album, ##in |
| alcohol | alcohol |
| allergy | all, ##er, ##gy |
| allopurinol | all, ##op, ##uri, ##no, ##l |
| amantadine | am, ##ant, ##adi, ##ne |
| amenorrhoea | am, ##eno, ##rr, ##hoe, ##a |
| amiodarone | am, ##io, ##dar, ##one |
| amyloidoses | am, ##yl, ##oid, ##ose, ##s |
| anemia | an, ##emia |
| aneurysm | an, ##eur, ##ys, ##m |
| angina | an, ##gin, ##a |
| anorexia | an, ##ore, ##xia |
| anosmia | an, ##os, ##mia |
| anovulation | an, ##ov, ##ulation |
| anoxia | an, ##ox, ##ia |
| antabuse | ant, ##ab, ##use |
| aphonia | a, ##phon, ##ia |
| appendicitis | app, ##end, ##icit, ##is |
| arteriosclerosis | art, ##eri, ##os, ##cle, ##rosis |
| arthralgia | art, ##hra, ##l, ##gia |
| arthritis | art, ##hr, ##itis |
| aspirin | as, ##pi, ##rin |
| asthma | as, ##th, ##ma |
| ataxia | at, ##ax, ##ia |
| atenolol | ate, ##no, ##lo, ##l |
| atherosclerosis | at, ##her, ##os, ##cle, ##rosis |
| ativan | at, ##iva, ##n |
| avandia | a, ##van, ##dia |
| avelox | a, ##vel, ##ox |
| avitaminosis | a, ##vi, ##tam, ##ino, ##sis |
| babesiosis | babe, ##sio, ##sis |
| bacitracin | b, ##ac, ##it, ##rac, ##in |

| | |
|---|---|
| bandemia | band, ##emia |
| bedwetting | bed, ##we, ##tting |
| blanching | b, ##lan, ##ching |
| bleomycin | b, ##leo, ##my, ##cin |
| blepharospasm | b, ##le, ##pha, ##ros, ##pas, ##m |
| bronchitis | br, ##on, ##chi, ##tis |
| brucellosis | br, ##uce, ##llo, ##sis |
| cachexia | cache, ##xia |
| calamine | ca, ##lam, ##ine |
| calan | ca, ##lan |
| candidiasis | can, ##di, ##dia, ##sis |
| carboplatin | car, ##bo, ##p, ##lat, ##in |
| cardiomyopathies | card, ##io, ##my, ##op, ##ath, ##ies |
| cardiomyopathy | card, ##io, ##my, ##op, ##athy |
| carsickness | cars, ##ick, ##ness |
| catapres | cat, ##ap, ##res |
| cataract | cat, ##ara, ##ct |
| cataracts | cat, ##ara, ##cts |
| catatonia | cat, ##aton, ##ia |
| catch | catch |
| cefaclor | c, ##ef, ##ac, ##lor |
| cefazolin | c, ##ef, ##az, ##olin |
| cefepime | c, ##ef, ##ep, ##ime |
| cefoxitin | c, ##ef, ##ox, ##iti, ##n |
| chills | chill, ##s |
| cholestasis | ch, ##ole, ##sta, ##sis |
| cholestyramine | ch, ##ole, ##sty, ##ram, ##ine |
| chyluria | ch, ##yl, ##uria |
| cipro | c, ##ip, ##ro |
| cirrhosis | c, ##ir, ##r, ##hos, ##is |
| cisplatin | c, ##is, ##p, ##lat, ##in |
| clonus | c, ##lon, ##us |
| clubbing | club, ##bing |
| cluttering | c, ##lut, ##tering |
| coccidioidomycosis | co, ##cci, ##dio, ##ido, ##my, ##cos, ##is |
| codeine | code, ##ine |
| colchicine | co, ##l, ##chi, ##cine |
| colitis | co, ##lit, ##is |
| comatose | coma, ##tos, ##e |
| constipation | con, ##st, ##ip, ##ation |
| convulsion | con, ##vu, ##ls, ##ion |
| corkscrewing | co, ##rks, ##cre, ##wing |
| cortisone | co, ##rt, ##ison, ##e |

| | |
|---|---|
| coumadin | co, ##uma, ##din |
| cozaar | co, ##za, ##ar |
| cromolyn | c, ##rom, ##oly, ##n |
| crowning | crown, ##ing |
| cyanosis | c, ##yan, ##osis |
| deafness | deaf, ##ness |
| dehydration | de, ##hy, ##dra, ##tion |
| dementia | dem, ##ent, ##ia |
| dementias | dem, ##ent, ##ias |
| dermatitis | der, ##mat, ##itis |
| dermatomyositis | der, ##mat, ##omy, ##os, ##itis |
| dexamethasone | de, ##xa, ##met, ##has, ##one |
| diabetes | diabetes |
| diarrhea | di, ##ar, ##r, ##hea |
| digoxin | dig, ##ox, ##in |
| dilantin | di, ##lant, ##in |
| diovan | di, ##ova, ##n |
| dizziness | di, ##zzi, ##ness |
| drooling | d, ##roo, ##ling |
| dulcolax | du, ##l, ##cola, ##x |
| duragesic | du, ##rage, ##si, ##c |
| dysentery | d, ##ys, ##enter, ##y |
| dyslipidemia | d, ##ys, ##lip, ##ide, ##mia |
| dyspnea | d, ##ys, ##p, ##nea |
| dysuria | d, ##ys, ##uria |
| earache | ear, ##ache |
| emaciation | em, ##ac, ##iation |
| enalapril | en, ##ala, ##p, ##ril |
| encephalitis | en, ##ce, ##pha, ##lit, ##is |
| epilepsy | e, ##pile, ##psy |
| erythema | er, ##yt, ##hem, ##a |
| erythromycin | er, ##yt, ##hr, ##omy, ##cin |
| esmolol | es, ##mo, ##lo, ##l |
| ethanol | ethanol |
| exophthalmos | ex, ##op, ##ht, ##hal, ##mos |
| fatigue | fatigue |
| fibrillation | fi, ##bri, ##lla, ##tion |
| fishmouth | fish, ##mouth |
| flatulence | flat, ##ule, ##nce |
| flushing | flush, ##ing |
| fosamax | f, ##osa, ##max |
| garlic | garlic |
| gastroenteritis | gas, ##tro, ##enter, ##itis |

| | |
|---|---|
| giardiasis | g, ##iard, ##ias, ##is |
| glaucoma | g, ##lau, ##com, ##a |
| glomerulosclerosis | g, ##lo, ##mer, ##ulos, ##cle, ##rosis |
| glucophage | g, ##lu, ##co, ##pha, ##ge |
| glyburide | g, ##ly, ##bur, ##ide |
| goiter | go, ##iter |
| gonorrhea | go, ##nor, ##r, ##hea |
| grimaces | grim, ##ace, ##s |
| haemorrhoids | ha, ##em, ##or, ##r, ##ho, ##ids |
| halitosis | ha, ##lit, ##osis |
| headache | headache |
| heartburn | heart, ##burn |
| hematemesis | hem, ##ate, ##mes, ##is |
| hemiballismus | hem, ##iba, ##llis, ##mus |
| hemicrania | hem, ##ic, ##rani, ##a |
| hemiplegia | hem, ##ip, ##leg, ##ia |
| hemochromatosis | hem, ##och, ##roma, ##tosis |
| hemoglobinopathy | hem, ##og, ##lo, ##bino, ##pathy |
| hemophilia | hem, ##op, ##hil, ##ia |
| hemoptysis | hem, ##op, ##ty, ##sis |
| heparin | he, ##par, ##in |
| hepatitis | he, ##pa, ##titis |
| hepatomegaly | he, ##pa, ##tom, ##eg, ##aly |
| hepatosplenomegaly | he, ##pa, ##tos, ##ple, ##no, ##me, ##gal, ##y |
| hernia | her, ##nia |
| hernias | her, ##nia, ##s |
| herpes | her, ##pes |
| histoplasmosis | his, ##top, ##las, ##mos, ##is |
| hunger | hunger |
| hyperacusis | h, ##yper, ##ac, ##us, ##is |
| hyperemesis | h, ##yper, ##em, ##esis |
| hyperesthesia | h, ##yper, ##est, ##hesia |
| hyperextension | h, ##yper, ##ex, ##tens, ##ion |
| hyperglycemia | h, ##yper, ##gly, ##ce, ##mia |
| hyperlipidemia | h, ##yper, ##lip, ##ide, ##mia |
| hyperoxia | h, ##yper, ##ox, ##ia |
| hypersomnolence | h, ##yper, ##so, ##m, ##no, ##len, ##ce |
| hyperthyroidism | h, ##yper, ##thy, ##roid, ##ism |
| hypoproteinemia | h, ##y, ##pop, ##rote, ##ine, ##mia |
| hypothyroidism | h, ##y, ##pot, ##hy, ##roid, ##ism |
| incontinence | in, ##con, ##tine, ##nce |
| infertility | in, ##fer, ##tility |
| influenza | in, ##fluenza |

| | |
|---|---|
| influenzae | in, ##fluenza, ##e |
| insulin | insulin |
| iron | iron |
| ischemia | is, ##che, ##mia |
| isosorbide | is, ##oso, ##rb, ##ide |
| ketonuria | k, ##eton, ##uria |
| lasix | las, ##ix |
| lethargy | let, ##har, ##gy |
| leukopenia | le, ##uk, ##ope, ##nia |
| levaquin | le, ##va, ##quin |
| lidocaine | lid, ##oc, ##aine |
| lipitor | lip, ##itor |
| lisinopril | l, ##isi, ##no, ##p, ##ril |
| loperamide | lo, ##per, ##ami, ##de |
| lovastatin | lo, ##vas, ##tat, ##in |
| malaria | malaria |
| malnutrition | ma, ##ln, ##utrition |
| mannerism | manner, ##ism |
| mannitol | man, ##ni, ##to, ##l |
| mastodynia | mast, ##ody, ##nia |
| medrol | me, ##dr, ##ol |
| meningism | men, ##ing, ##ism |
| meningitis | men, ##ing, ##itis |
| metatarsalgia | meta, ##tars, ##al, ##gia |
| methadone | met, ##had, ##one |
| methotrexate | met, ##hot, ##re, ##xa, ##te |
| mittelschmerz | mit, ##tel, ##sch, ##mer, ##z |
| morphine | m, ##or, ##phine |
| motrin | m, ##ot, ##rin |
| mycoses | my, ##cos, ##es |
| mycosis | my, ##cos, ##is |
| myelosuppression | my, ##elo, ##su, ##pp, ##ression |
| myopathy | my, ##op, ##athy |
| myositis | my, ##os, ##itis |
| narcan | na, ##rca, ##n |
| nausea | nausea |
| nephritis | ne, ##ph, ##rit, ##is |
| neuralgia | neural, ##gia |
| neuropathy | ne, ##uro, ##pathy |
| nitroglycerine | ni, ##tro, ##gly, ##cer, ##ine |
| nocturia | no, ##ct, ##uria |
| nystagmus | n, ##ys, ##tag, ##mus |
| obesity | o, ##besity |

| | |
|---|---|
| opisthotonus | op, ##ist, ##hot, ##on, ##us |
| osteoporosis | o, ##ste, ##op, ##oro, ##sis |
| otitis | o, ##titis |
| overeating | over, ##eat, ##ing |
| pain | pain |
| pallor | p, ##allo, ##r |
| pancreatitis | pan, ##cre, ##ati, ##tis |
| parasitemia | parasite, ##mia |
| paresis | par, ##esis |
| penicillin | pen, ##ici, ##llin |
| pepcid | p, ##ep, ##cid |
| peritonitis | per, ##ito, ##ni, ##tis |
| phenobarbital | p, ##hen, ##ob, ##ar, ##bit, ##al |
| photopsia | photo, ##ps, ##ia |
| photosensitization | photos, ##ens, ##iti, ##zation |
| plague | plague |
| plavix | p, ##lav, ##ix |
| pneumonia | pneumonia |
| pneumoniae | pneumonia, ##e |
| polydipsia | p, ##oly, ##di, ##ps, ##ia |
| polyuria | p, ##oly, ##uria |
| prednisolone | pre, ##dn, ##is, ##olo, ##ne |
| prilosec | p, ##ril, ##ose, ##c |
| probenecid | probe, ##ne, ##cid |
| propofol | prop, ##of, ##ol |
| protamine | pro, ##tamine |
| proteinuria | protein, ##uria |
| prozac | pro, ##zac |
| psoriasis | ps, ##oria, ##sis |
| pyorrhea | p, ##yo, ##rr, ##hea |
| rabies | r, ##abi, ##es |
| rales | r, ##ales |
| regurgitation | re, ##gu, ##rg, ##itation |
| reticulocytosis | re, ##tic, ##ulo, ##cy, ##tosis |
| rheumatism | r, ##he, ##uma, ##tism |
| rhonchi | r, ##hon, ##chi |
| robitussin | r, ##ob, ##it, ##uss, ##in |
| rogaine | r, ##oga, ##ine |
| sandimmune | sand, ##im, ##mu, ##ne |
| schistosomiasis | s, ##chi, ##sto, ##so, ##mia, ##sis |
| sciatica | s, ##cia, ##tica |
| scleroderma | s, ##cle, ##rod, ##er, ##ma |
| seasickness | seas, ##ick, ##ness |

| | |
|---|---|
| seizures | seizure, ##s |
| septicemia | se, ##ptic, ##emia |
| sinemet | sin, ##em, ##et |
| singulair | sing, ##ula, ##ir |
| sleeplessness | sleep, ##lessness |
| sluggishness | s, ##lug, ##gis, ##hn, ##ess |
| smallpox | small, ##pox |
| snoring | s, ##nor, ##ing |
| spasm | spa, ##sm |
| spiriva | s, ##pi, ##ri, ##va |
| starvation | starvation |
| stridor | s, ##tri, ##dor |
| syncope | s, ##ync, ##ope |
| synthroid | s, ##ynth, ##roid |
| syphilis | s, ##y, ##phi, ##lis |
| tamiflu | ta, ##mi, ##f, ##lu |
| thalassemia | th, ##ala, ##sse, ##mia |
| thirsty | thirst, ##y |
| thrombocytopenia | th, ##rom, ##bo, ##cy, ##top, ##enia |
| thromboembolism | th, ##rom, ##boe, ##mbo, ##lis, ##m |
| thrombophilias | th, ##rom, ##bo, ##phi, ##lia, ##s |
| thrombus | th, ##rom, ##bus |
| tiredness | tired, ##ness |
| toothache | tooth, ##ache |
| toprol | top, ##rol |
| torticollis | to, ##rt, ##ico, ##llis |
| trembling | trembling |
| tremor | t, ##rem, ##or |
| tuberculosis | tuberculosis |
| tylenol | t, ##yle, ##no, ##l |
| ultram | ultra, ##m |
| uremia | u, ##rem, ##ia |
| urolithiasis | u, ##rol, ##ith, ##ias, ##is |
| vaccinia | v, ##ac, ##cini, ##a |
| vasculitis | v, ##as, ##cu, ##lit, ##is |
| vertigo | ve, ##rt, ##igo |
| virilization | v, ##iri, ##li, ##zation |
| vomiting | vomit, ##ing |
| weakness | weakness |
| wellbutrin | well, ##but, ##rin |
| welts | we, ##lts |
| wheezing | w, ##hee, ##zing |
| xanax | x, ##ana, ##x |

| | |
|---|---|
| xenical | x, ##eni, ##cal |
| zantac | z, ##ant, ##ac |
| zithromax | z, ##ith, ##roma, ##x |
| zocor | z, ##oc, ##or |
| zofran | z, ##of, ##ran |
| zoloft | z, ##olo, ##ft |
| zoonosis | zoo, ##nosis |
| zovirax | z, ##ov, ##ira, ##x |
